# Supplementary material for: Learning the Number of Neurons in Deep Networks
Source: arXiv:1611.06321 source file (2018-10-11)
Supplement: Supplementary file 1 [file supplementalmaterial.tex]

\section{Additional Experiments}

\paragraph{Places2-401:} We now turn to the second large-scale image recognition dataset, Places 2. For this experiment, we focused on the Dec$_8$-640 architecture, trained with either the group sparsity regularizer or the sparse group Lasso one. Figure~\ref{fig:DecOnPlaces} summarizes our results and compares them with several baselines. These results are consistent with those obtained on ImageNet. The group sparsity regularizer reduces the total number of parameters by more than 10\%, and the sparse group Lasso yields an even greater reduction of $10\%$ of the neurons, which amounts to more than 18\% of the parameters. In both cases, the resulting network also leads to an improvement in top-1 accuracy. Importantly, this lets us outperform the current state-of-the-art on this dataset, even without using any advanced data augmentation technique such as color corrections or multiple crops at test time as in~\citep{ResNet2015,Krizhevsky_imagenetclassification}.
  
 \begin{figure}[t!]
 \begin{center}
 \begin{minipage}[t]{.335\linewidth}
 \vspace{0pt}
 \centering
\hspace{-0.3cm}\includegraphics[width=\textwidth]{./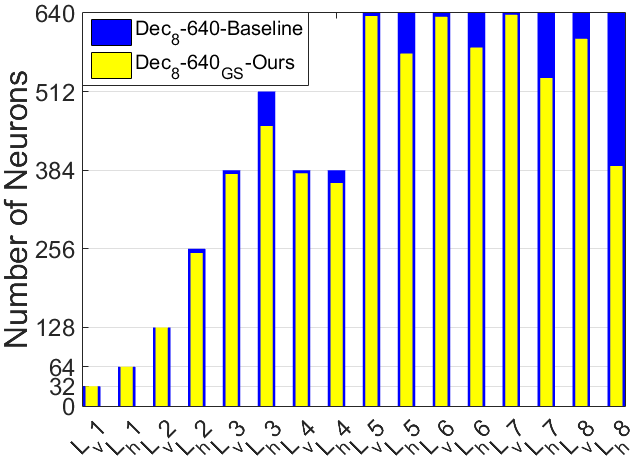}
 \end{minipage}%
 \begin{minipage}[t]{.65\linewidth}
 \vspace{0pt}
 \centering
 \begin{tabular}{ cc }%
\hspace{-0.25cm}\begin{tabular}{ |l|c|c| }%
      \hline%
      \multicolumn{3}{|c|}{Dec$_8$-$640$ on Places2 (in \%)} \\%
      \hline \hline 
     &\multicolumn{1}{c|}{SGL}&\multicolumn{1}{c|}{GS} \\%
     \hline
    neurons& 10.08&8.05\\
    group param& 11.40 & 9.18\\
    total param& 17.99 & 9.18\\
    total induced & 18.53&\ADDED{14.79}\\
    \hline
    accuracy gap & 1.31&1.88\\
    \hline      
    \end{tabular}%
&\hspace{-0.25cm}\begin{tabular}{ |l|c| }%
      \hline%
      \multicolumn{2}{|c|}{Top-1 acc (\%) on Places2}\\%
      \hline \hline
%	AlexNetOWTBn& 44.5\\
%	AlexNetOWTBn$^C$& 41.1\\
    BNet& 44.0\\
    BNet$^C$& 43.1\\
	Dec$_8$ & 46.6\\
    Dec$_8$-640 & 46.8\\
	\hline      
	Ours-Dec$_8$-640$_{GS}$ & 47.6\\
  	Ours-Dec$_8$-640$_{SGL}$ & 47.3\\
\hline      
    \end{tabular}\\
\end{tabular}%
 \end{minipage}
 \end{center}
 \vspace{-0.3cm}
 \caption{Experimental results on Places2-401 using Dec$_8$-$640$. From left to right, we show the reduction in number of neurons for each layer, the percentage of zeroed-out neuron/parameters, and the top-1 accuracy, compared to several baselines. Note that we achieve a significant reduction in number of parameters and, importantly, outperform the state-of-the-art on this dataset.}
 \label{fig:DecOnPlaces} 
 \end{figure}
